# Supplementary material for: Search for An Annual Modulation in Three Years of CoGeNT Dark Matter Detector Data
Source: arXiv:1401.3295 ancillary file (2014-01-14)
Supplement: Supplementary file 1 [file read_me.pdf]

## **Brief description of data file format and usage (Databases S1, S2, S3)**

As we have done in the past, we offer a public distribution of the data used in this analysis.

Events in databases S1 and S2 pass all cuts against microphonic events and spurious electronic pulses described in [1]. These events range in energy from 0.5 keVee to 3.2 keVee for S1, and 0.5 keVee to 12 keVee for S2. The lower boundary corresponds to the analysis threshold, upper boundaries to the maximum energy for which rise-time information is available in each channel [1]. These tab-delimited ASCII files contain three columns, corresponding to time-stamp, energy in keVee, and rise-time in  $\mu$ s. The time stamp is in elapsed seconds, with the first event taking place a few minutes after the midnight of Dec 4<sup>th</sup> 2009. Any analysis should take into account downtime periods [2] on days 68-74 (Feb 9<sup>th</sup>-15<sup>th</sup> 2010, inclusive), days 102-107 (March 15<sup>th</sup>-20<sup>th</sup> 2010, inclusive), and days 306-308 (Oct. 5<sup>th</sup>-7<sup>th</sup> 2010, inclusive). The last day in the pre-fire dataset is March 6<sup>th</sup> 2011, corresponding to a planned general outage at SUL [2]. Data acquisition was restarted post-fire on the midnight of June 7<sup>th</sup> 2011, following a three-month downtime, and was continuous (with negligible interruptions) until the last day included in this dataset, April 23<sup>rd</sup> 2013. Large blank gaps in the data correspond to the (removed) microphonic events accompanying the automatic LN2 refills that take place every 48 hours [1]. Events separated by less than 12 seconds are also removed as part of the microphonic rejection cuts [1], except for a small energy band around  $\sim$ 11 keV, to preserve the  $^{73}\text{As}$  activity in database S2 (there is an intermediate half-life of  $\sim$ 0.5 s involved in that decay). The negligible contribution from  $^{73}\text{As}$  is removed from database S1 by this cut.

Users of these datasets are advised to rely on database S1 for analyses below 3.2 keVee, given the more reliable energy calibration obtained there next to threshold. Similarly, the 8-bit data acquisition system employed [1] limits the smallest bin size that should be used in a binned energy analysis before spurious spectral features appear. A maximum of 256/2 energy bins is recommended for either dataset.

An expression for the resolution of the detector at low-energy is provided in [3] (notice relevant erratum in [4]), with parameters specific for this PPC being listed in [5]. Readers attempting a calculation of L-shell EC activities using the K-shell EC activities noticeable in database S2 should consult reference [6]. There are no corrections to be made to this calculation arising from different signal acceptances affecting database S1 and S2 (in the past we suggested making a small correction, but this originated on differences in the rise-time cuts applied to these two channels: databases S1 and S2 do not contain any rise-time cuts). The combined trigger plus microphonic cut efficiency (dashed line in the inset of Fig. 3 of [5]) should be kept in mind when analyzing these data. The table below can provide further guidance, listing relevant cosmogenic isotopes, their theoretical exchange-corrected L/K EC ratio from Bahcall [6], energy in keVee at which the L-shell EC peak centroid is expected (binding energy of the  $L_1$  shell), resolution at that energy, and half-life of the decay.

| isotope  | L/K EC ratio | BE L1 shell (keV) | sigma (keV) | T1/2 (days) |
|----------|--------------|-------------------|-------------|-------------|
| C0       | C1           | C2                | C3          | C4          |
| As 73    | 0.11000      | 1.4143            | 0.077656    | 80.000      |
| Ge 68    | 0.11400      | 1.2977            | 0.077008    | 271.00      |
| Ga 68    | 0.11000      | 1.1936            | 0.076426    | 271.00      |
| Zn 65    | 0.10800      | 1.0961            | 0.075877    | 244.00      |
| Ni 56    | 0.10200      | 0.92560           | 0.074906    | 5.9000      |
| Co 56,58 | 0.10200      | 0.84610           | 0.074449    | 71.000      |
| Co 57    | 0.10200      | 0.84610           | 0.074449    | 271.00      |
| Fe 55    | 0.10600      | 0.76900           | 0.074003    | 996.00      |
| Mn 54    | 0.10200      | 0.69460           | 0.073570    | 312.00      |
| Cr 51    | 0.10100      | 0.62820           | 0.073182    | 28.000      |
| Y 49     | 0.10000      | 0.56370           | 0.072803    | 330.00      |

Database S3 is not employed in the present analysis, but it is used in upcoming work [7]. It corresponds to fast electronic pulser events able to mimic, to a good extent, a radiation-induced pulse taking place within the bulk of the crystal [1,5]. This two-column ASCII file lists their energy in keVee and rise-time in  $\mu\text{s}$ , in this order, for a manual scan in pulser amplitude (energy). The rise-time already contains a 0.1  $\mu\text{s}$  correction described in [5]. This scan is similar to fixed-amplitude pulser runs discussed in Fig. 7 of [1]. Energies are not uniformly sampled in this manual scan, but a sufficiently large number of events is available at any energy. This file can be used by a reader interested in building energy-dependent rise-time distributions representative of events taking place in the bulk of this PPC crystal. This information can be used to approximate the signal acceptance for bulk events following the imposition of an arbitrary rise-time cut. In this respect, it is worth mentioning that the distribution of rise-time for bulk events presents a small tail extending towards large values of  $t_{10-90}$  not accounted for by a single log-normal fit [7]. This tail is visible in S3 pulser data, and simulations in [1]. The rise-time distribution of surface events is adequately described by a single log-normal distribution [7].

## References

- [1] C.E. Aalseth *et al.*, Phys. Rev. **D88**, 012002 (2013).
- [2] C.E. Aalseth *et al.*, Phys. Rev. Lett. **107**, 141301 (2011).
- [3] C.E. Aalseth *et al.*, Phys. Rev. Lett. **101**, 251301 (2008).
- [4] C.E. Aalseth *et al.*, Phys. Rev. Lett. **102**, 109903 (2009).
- [5] C.E. Aalseth *et al.*, Phys. Rev. Lett. **106**, 131301 (2011).
- [6] J.N. Bahcall, Phys. Rev. **132**, 362 (1963); W. Bambynek *et al.*, Rev. Mod. Phys. **49**, 77 (1977); W. Bambynek *et al.*, Rev. Mod. Phys. **49**, 961 (1977).
- [7] M. Bellis *et al.*, in preparation.
